# Supplementary material for: Riemannian Score-Based Generative Modelling
Source: arXiv:2202.02763 source file (2022-11-22)
Supplement: Supplementary file 1 [file frame_bundle.tex]

\subsection{Frame bundle and orthonormal frame bundle}
\label{sec:frame-bundle-orth}

We now introduce the concepts of frame bundle and orthonormal bundle over the
manifold $\M$. These concepts are useful to define stochastic processes on $\M$
using Euclidean stochastic processes. In particular, we will see that a Brownian
motion on the manifold can be linked to the Euclidean Brownian motion using the
orthonormal bundle. For any $x \in \M$, a frame at $x$ is an isomorphism
$f: \ \rset^d \to \mathrm{T}_x \M$. Note that $f$ is equivalent to the choice of
a basis in $\mathrm{T}_x \M$. We denote $\mathrm{F}_x \M$ the set of frames at
$p$. The frame bundle denoted $\FM$ is given by
$\FM = \sqcup_{x \in \M} \mathrm{F}_x \M$. The frame bundle can be given a
smooth structure and is therefore a $d + d^2$-dimensional manifold. Similarly,
for any $x \in \M$, an orthonormal frame at $x$ is a linear isometry
$f: \ \rset^d \to \mathrm{T}_x \M$. Note that $f$ is equivalent to the choice of
an orthonormal basis in $\mathrm{T}_x \M$. We denote $\mathrm{O}_p \M$ the set
of orthonormal frames at $p$. The orthonormal frame bundle denoted $\OM$ is
given by $\OM = \sqcup_{x \in \M} \mathrm{O}_x \M$. The orthonormal frame bundle
can be given a smooth structure and is therefore a $d + d(d-1)/2$-dimensional
manifold. We denote $\pi: \ \FM \to \M$ the smooth projection such that for any
$u = (x,f) \in \FM$, $\pi(u) = x$. Note that the restriction of $\pi$ to the
orthonormal bundle is also smooth.  Frame bundles and orthonormal bundles are
primary examples of principal bundles and we refer to \textcite{kolar2013natural}
for more details.

One key element of frame bundles and orthonormal bundles is their link with the
connections on $\M$. Let $u = (x, f) \in \FM$ and
$U \in \mathrm{T}_u \mathrm{F}M$. $U$ is said to be vertical if there exists a
smooth curve $u: \ \ccint{0,1} \to \FM$ such that for any $t \in \ccint{0,1}$,
$\pi(u(t)) = x$ and $\dot u(0) = U$. We say that $U$ is tangent to the fibre
$\mathrm{F}_{\pi(u)}\M$. The space of vertical tangent vectors is called the
vertical space and is denoted $\mathrm{V}_u \FM$. We have that
$\mathrm{dim}(\mathrm{V}_u \mathrm{F}\M) = d^2$. We now define the horizontal
space as follows. Let $u: \ \ccint{0,1} \to \FM$ be a smooth curve. We say that
$u = (f,x)$ is horizontal if for any $t \in \ccint{0,1}$ and
$i \in \{1, \dots, d\}$, $\nabla_{\dot x} (f e_i)(t) = 0$, where
$\{e_i\}_{i=1}^d$ is the canonical basis of $\rset^d$. In other words, the
horizontal curve corresponds to the parallel transport of a frame along a smooth
curve in $\M$. Let $u = (x, f) \in \FM$ and $U \in \mathrm{T}_u
\mathrm{F}M$. $U$ is said to be horizontal if there exists a smooth horizontal
curve $u: \ \ccint{0,1} \to \FM$ such that $\dot u(0) = U$. The space of
horizontal tangent vectors is called the horizontal space and is denoted
$\mathrm{H}_u \FM$. Let $v \in \rset^d$, we define the vector field
$H_v \in \mathcal{X}(\FM)$ such that for any $u \in \FM$, $H_v(u) = \dot u(0)$
with $\gamma=(x,f): \ \ccint{0,1} \to \FM$ a smooth curve on $\FM$ such that
$\dot x(0) = e(0)v$ and $\gamma(0) = u$. The existence of $H_v$ for any
$v \in \rset^d$ is discussed in \citet[p.69-70]{kobayashi1963foundations} and
$H_v$ is called the horizontal lift of $v$. For any $i \in \{1, \dots, d\}$ we
denote $H_i = H_{e_i}$ where $\{e_i\}_{i=1}^d$ is the canonical basis of
$\rset^d$. In particular, since any horizontal curve is entirely specified by
$\gamma(0) = (x(0), f(0))$ and $\dot{x}(0)$, we get that
$\mathrm{dim}(\mathrm{H}_u \FM) = d$ for any $u \in \FM$.

Consider a connection $\nabla$ on $\M$. Note that for any $u = (x,f) \in \FM$, we have
$\mathrm{T}_u \FM = \mathrm{T}_u \M \oplus \mathrm{V}_u \FM$. In local
coordinates $\{x_i\}_{i=1}^d$, we denote $\{X_i\}_{i=1}^d$ a basis of
$\mathrm{T}_x \M$. For any $j \in \{1, \dots, j\}$, there exist
$\{f_{i,j}\}_{i=1}^d$ such that $f e_j = \sum_{i=1}^d f_{i,j} X_i$ (note that
$\{f_{i,j}\}_{1 \leq i,j \leq d}$ can be interpreted as the matrix transforming
a vector of $\rset^d$ into a vector of $\mathrm{T}_x\M$ expressed in the basis
$\{X_i\}_{i=1}^d$). In particular, we have that
$\{x_k, f_{i,j}\}_{1 \leq i,j, k \leq d}$ are local coordinates for $\FM$. We
denote by $\{X_k, X_{i,j}\}_{1 \leq i,j,k \leq d}$ the associated basis in
$\mathrm{T}_u \FM$ for any $u \in \msu$, where $\msu$ is an open subset of $\FM$
on which the local coordinates are well-defined. Leveraging properties of
parallel transport, we have that for any $j \in \{1, \dots, d\}$ and $u \in \msu$
\begin{equation}
  \label{eq:horizontal_lift}
  \textstyle{ H_j(u) = \sum_{i=1}^d f_{i,j} X_i - \sum_{\ell, m=1}^d \{ \sum_{i, k=1}^d f_{i,j} f_{k,m} \Gamma_{i,k}^\ell\} X_{\ell,m}  ,}
\end{equation}
where we recall that $\{\Gamma_{i,j}^k\}_{1 \leq i,j,k \leq d}$ are the
Christoffel symbols of the connection in local coordinates.  In particular, it
is clear that for any $u \in \FM$, $\{H_i(u)\}_{i=1}^d$ is a basis of
$\mathrm{H}_u \FM$ and that $\mathrm{H}_u \FM \cap \mathrm{V}_u \FM = \{0\}$,
hence $\mathrm{T}_u \FM = \mathrm{H}_u \FM \oplus \mathrm{V}_u \FM$. Using
\cref{eq:horizontal_lift} we have that the horizontal space is entirely defined
by the connection $\nabla$. Reciprocally, any smooth linear complement of the
vertical space gives rise to a connection \cite[see][Section
11.11]{kolar2013natural}.

We now illustrate how we can go from a smooth curve on $\M$ (equipped with a
connection $\nabla$) to a smooth curve on $\rset^d$. First, let
$x: \ \ccint{0,1} \to \M$ be a smooth curve on manifold. Define
$f(0) \in \mathrm{F}_{x(0)} \M$ and consider $u: \ \ccint{0,1} \to \FM$ the
smooth horizontal curve associated with $x$ and starting frame $f(0)$. Now
consider the antidevelopment of $u$ given by the smooth curve
$z: \ \ccint{0,1} \to \rset^d$ such that for any $t \in \ccint{0,t}$
\begin{equation}
  \textstyle{ z(t) = \int_0^t f(s)^{-1} \dot x(s) \rmd s   . }
\end{equation}
We now show how a smooth curve on $\rset^d$ gives rise to a smooth curve in
$\M$. First, note that for any $t \in \ccint{0,1}$, we have that
$\dot u (t) = \sum_{i=1}^d H_i(u(t)) \dot z_i(t)$. Hence, specifying $u(0)$ any
smooth curve $z$ on $\rset^d$ is associated to a smooth curve on $\FM$. We
obtain a smooth curve on $\M$ by considering $x = \pi(u)$. In the next section,
we present similar ideas when smooth curves are replaced by semimartingales.

\subsection{Horizontal lift and stochastic development}
\label{sec:horiz-lift-stoch}

We are now ready to present the notion of horizontal semimartingale, which is
key to draw the link between semimartingales on $\M$ and semimartingales on
$\rset^d$. We follow the presentation of \citet[Section
2.3]{hsu2002stochastic}. Again, we consider a filtered probability space
$(\Omega, (\mcf_t)_{t \geq 0}, \Pbb)$. All the semimartingales we consider are
defined w.r.t this filtered probability space. We assume that the manifold $\M$
is equipped with a connection $\nabla$.

\begin{definition}[Stochastic development]
  Let $(\bfZ^{1:d}_t)_{t \geq 0} = \{(\bfZ_t^i)_{t \geq 0}\}_{i=1}^d$ be a
  collection of real-valued semimartingales.  Let $(\bfU_t)_{t \geq 0}$ be the
  $\FM$ semimartingale solution of $\SDE(H^{1:d}, \bfZ^{1:d}, \bfU_0)$ with
  $H^{1:d} = \{H_i\}_{i=1}^d$. $(\bfU_t)_{t \geq 0}$ is called the \emph{stochastic
    development} of $\bfZ^{1:d}$ on $\FM$. Similarly, the $\M$-valued
  semimartingale $(\bfX_t)_{t \geq 0} = (\pi(\bfU_t))_{t \geq 0}$ is called the
  \emph{stochastic development} of $\bfZ^{1:d}$ on $\M$.
\end{definition}

The previous definition allows to transfer a semimartingale on $\rset^d$ to a
semimartingale on $\M$ in an \emph{intrinsic} manner. Reciprocally, we also aim
at transferring a semimartingale on $\M$ to a semimartingale on $\rset^d$.

\begin{definition}[Horizontal lift and antivelopment]
  Let $(\bfX_t)_{t \geq 0}$ be a $\M$-valued semimartingale. If there exist a
  $\FM$-valued semimartingale $(\bfU_t)_{t \geq 0}$ and
  $(\bfZ^{1:d}_t)_{t \geq 0} = \{(\bfZ_t^i)_{t \geq 0}\}_{i=1}^d$ a collection
  of real-valued semimartingales such that
  $(\bfX_t)_{t \geq 0} = (\pi(\bfU_t))_{t \geq 0}$ and $(\bfU_t)_{t \geq 0}$ is
  solution of $\SDE(H^{1:d}, \bfZ^{1:d}, \bfU_0)$ with
  $H^{1:d} = \{H_i\}_{i=1}^d$ then $(\bfU_t)_{t \geq 0}$ is called the
  \emph{horizontal lift} of $(\bfX_t)_{t \geq 0}$ and
  $(\bfZ^{1:d}_t)_{t \geq 0}$ the \emph{antidevelopment} of
  $(\bfX_t)_{t \geq 0}$.
\end{definition}

The existence of an horizontal lift and an antidevelopment is not
trivial. Considering the Nash embedding theorem 
\citep[see for example][]{gunther1991isometric}, it is possible to show the existence
and uniqueness of these processes (up to initialization). Without loss of
generality, we can then assume that $\M \subset \rset^p$ and for any $x \in \M$,
$\mathrm{T}_x \M \subset \rset^p$ with $p \geq d(d+1)/2$ (and
$p \leq \max(d(d+5)/2, d(d+3)/2+5)$). For any $x \in \M$, we denote
$P(x): \ \rset^p \to \mathrm{T}_x \M$ the projection operator. In addition for
any $x \in \M$, we denote $\{P_i(x)\}_{i=1}^p = \{P(x) e_i\}_{i=1}^p$, where
$\{e_i\}_{i=1}^p$ is the canonical basis of $\rset^p$. Note that
$\{P_i\}_{i=1}^p \in \XM^p$. In addition for any $x \in \M$ we denote
$\{x^i\}_{i=1}^p$ its coordinates in $\rset^p$, \ie \ for any
$i \in \{1, \dots, p\}$, $x^i = \langle x, e_i \rangle$. In particular, if
$(\bfX_t)_{t \geq 0}$ is a $\M$-valued process then for any
$i \in \{1, \dots, p\}$,
$(\bfX_t^i)_{t \geq 0} = (\langle \bfX_t, e_i \rangle)_{t \geq 0}$ is a
real-valued process. If $(\bfX_t)_{t \geq 0}$ is a $\M$-valued semimartingale
then it is the solution of $\SDE(\{P_i\}_{i=1}^p, \{\bfX^i\}_{i=1}^p, \bfX_0)$
\cite[see][Lemma 2.3.3]{hsu2002stochastic}. Then, a candidate for the horizontal
lift of $(\bfX_t)_{t \geq 0}$ is given by
$(\bfU_t)_{t \geq 0}=(\bfX_t, \bfE_t)_{t \geq 0}$ solution of
$\SDE(\{P_i^\star\}_{i=1}^p, \{\bfX^i\}_{i=1}^p, \bfU_0)$, where for any
$i \in \{1,\dots,p\}$, $P_i^\star(u) = H_{f^{-1}P_i(\pi(u))}(u)$ and
$\bfX_0 = \pi(\bfU_0)$. We have that $(\bfU_t)_{t \geq 0}$ is the stochastic
development of $\{(\bfZ_t^i)_{t \geq 0}\}_{i=1}^d$ where for any $t \geq 0$,
$\bfZ_t = \sum_{i=1}^p \int_0^t \bfE_s^{-1} P_i(\bfX_s) \circ \rmd \bfX_s^i$
 \cite[see][Theorem 2.3.4]{hsu2002stochastic}. Finally, we have that given
$\bfU_0$, $(\bfU_t)_{t \geq 0}$ is the unique horizontal lift of
$(\bfX_t)_{t \geq 0}$ and $(\bfZ_t)_{t \geq 0}$ is the unique antidevelopment of
$(\bfX_t)_{t \geq 0}$ \cite[see][Theorem 2.3.5]{hsu2002stochastic}.

%%% Local Variables:
%%% mode: latex
%%% TeX-master: "../main"
%%% End:
