# Supplementary material for: Riemannian Score-Based Generative Modelling
Source: arXiv:2202.02763 source file (2022-11-22)
Supplement: Supplementary file 2 [file schrodinger.tex]

\section{Schr\"odinger Bridges on Manifolds}
\label{sec:schrodinger}

%\valentin{no compelling examples for conditional sampling... Maybe in physics?}

\paragraph{Dynamical Schr\"odinger bridges}
We briefly recall the notion of dynamical Schr\"odinger bridge
\citep{leonard2012schrodinger,chen2016entropic,vargas2021solving,debortoli2021neurips,chen2021likelihood}. We
consider a reference path probability measure
$\Pbb \in \Pens(\rmc(\ccint{0,T}, \M))$. In practice, we set $\Pbb$ to be the
distribution of the Brownian motion $(\bfB_t^\M)_{t \in \ccint{0,T}}$ such that
$\bfB_0^\M$ has distribution $\pizero$, the target data distribution. Then, we consider
the \emph{dynamical Schr\"odinger bridge problem}
\begin{equation}
  \Qbb^\star = \argmin \ensembleLigne{\KL{\Qbb}{\Pbb}}{\Qbb \in \Pens(\ccint{0,T}, \M), \ \Qbb_0 = \pizero, \ \Qbb_T = \piinv} . 
\end{equation}
The solution $\Qbb^\star$ is called the Schr\"odinger Bridge (SB).  Note that if
$\Qbb^\star$ is associated with a backward process
$(\bfY_t^\star)_{t \in \ccint{0,T}}$, then we can obtain a generative model as
follows. First sample from $\piinv = \mathcal{L}(\bfY^\star_T)$ and then follow
the (backward) dynamics of $(\bfY^\star_t)_{t \in \ccint{0,T}}$. By definition, we obtain
that $\mathcal{L}(\bfY^\star_0) = \pizero$, the target distribution.

In practice however, the solution of the SB problem is approximated using the
Iterative Proportional Fitting (IPF) algorithm. Note that in discrete space the
IPF is also known as the Sinkhorn algorithm \citep{sinkhorn1967diagonal,peyre2019computational}. The
IPF defines a sequence of path probability measures
$(\Qbb^n)_{n \in \nset} \in (\Pens(\rmc(\ccint{0,T}, \M)))^\nset$, such that
$\Qbb^0 = \Pbb$ and for any $n \in \nset$
\begin{align}
  &\Qbb^{2n+1} = \argmin \ensembleLigne{\KL{\Qbb}{\Qbb^{2n}}}{\Qbb \in \Pens(\rmc(\ccint{0,T}, \M), \Qbb_T = \piinv}  , \\
  &\Qbb^{2n+2} = \argmin \ensembleLigne{\KL{\Qbb}{\Qbb^{2n+1}}}{\Qbb \in \Pens(\rmc(\ccint{0,T}, \M), \Qbb_0 = \pizero} .
\end{align}
Under mild assumptions on $\Pbb$, $\pizero$ and $\piinv$, we have that
$(\Qbb^n)_{n \in \nset}$ converges towards $\Qbb^\star$ \cite[see][]{nutz2022stability}.
In what follows, we propose an algorithm to
approximately sample from $(\Qbb^n)_{n \in \nset}$. In Euclidean state spaces,
\cite{debortoli2021neurips,vargas2021solving,chen2021likelihood} have proposed
an algorithm based on time-reversal to compute the IPF. We now extend these
techniques to the case of Riemannian manifolds.

\paragraph{Riemannian Diffusion Schr\"odinger Bridge}

We propose Riemannian Diffusion Schr\"odinger Bridge (RDSB) an extension of
Diffusion Schr\"odinger Bridge \cite{debortoli2021neurips} to approximate
solutions of SB problems. First, we connect the iterates
$(\Qbb^n)_{n \in \nset}$ with diffusion processes on $\M$.

\begin{proposition}
  \label{prop:continuous_schro}
  Let $\Pbb$ be the path measure of the Brownian motion initialized at $\piinv$.
  Assume that for any $n \in \nset$, $\KL{\Qbb^n}{\Pbb}< +\infty$ and that for
  any $t \in \ccint{0,T}$ and $n \in \nset$, $\Qbb^n_t$ admits a smooth positive
  density w.r.t.\ $\piinv$. Then, for any $n \in \nset$ we have:
  \begin{enumerate}[wide, labelwidth=!, labelindent=0pt, label=(\alph*)]
  \item $R(\Qbb^{2n+1})$ solves the martingale problem with generator $\generator^{2n+1}(t,u) = \langle \nabla u, b_{T-t}^n \rangle_\M + \tfrac{1}{2} \Delta_\M u$;
  \item $\Qbb^{2n+2}$ solves the martingale problem with generator $\generator^{2n+2}(t,u) = \langle \nabla u, f_{t}^{n+1} \rangle_\M + \tfrac{1}{2} \Delta_\M u$;    
  \end{enumerate}
  where for any $n \in \nset$, $t \in \ccint{0,T}$ and 
  $x \in \rset^d$, $b^{n}_t( x) = -f^{n}_t(x) + \nabla \log p^{n}_t(x)$, 
  $f^{n+1}_t(x) = -b^n_t(x) + \nabla \log q^n_t(x)$, with $f^0_t(x) = 0$, and $p^n_t$, $q_t^n$
  the densities of $\Qbb^{2n}_t$ and  $\Qbb_t^{2n+1}$.
\end{proposition}

\begin{proof}
  The proof is similar to \citet[Proposition 6]{debortoli2021neurips} using
  \Cref{thm:time_reversal_manifold} instead of \citet[Theorem
  4.19]{cattiaux2021time}
\end{proof}

In particular, we have that $\Qbb^1$ is the diffusion process associated with
RSGM, \ie \ the time-reversal of the Brownian motion initialized at
$\piinv$. Hence, $\Qbb^{2n+1}$ for $n \in \nset$ with $n \geq 1$ can be seen as
a refinement of $\Qbb^1$. In the next proposition, we show that the drift term
of the diffusion processes associated with $(\Qbb^n)_{n \in \nset}$ can be
approximated leveraging score-based techniques.

\begin{proposition}
  \label{prop:loss_implicit_explicit}
  Let $(\bfX_t)_{t \in \ccint{0,T}}$ be a $\M$-valued process with distribution
  $\Pbb \in \Pens(\rmc(\ccint{0,T}, \M))$ such that for any $t \in \ccint{0,T}$,
  $\bfX_t$ admits a positive density $p_t \in \rmc^\infty(\M)$
  w.r.t.\ $\piinv$. Let $s: \ \ccint{0,T} \to \XM$. For any $t \in \ccint{0,T}$
  and $x \in \M$, let
  \begin{equation}
    b(t,x) = -f(t,x) + g(t, \bfX_t)^2\nabla \log p_t(x) . 
  \end{equation}
  Then, for any $t \in \ccint{0,T}$, we have that
  \begin{equation}
    b(t, \cdot) = \argmin \ensembleLigne{\expeLigne{\tfrac{1}{2}\normLigne{f(t, \bfX_t) + r(\bfX_t)}^2 + g(t, \bfX_t)^2\dive(r)(\bfX_t)}}{r \in \mathrm{L}^2(\Pbb_t)} . 
  \end{equation}
\end{proposition}

\begin{proof}
  Let $t \in \ccint{0,T}$. First, we have for any $x \in \M$
  \begin{align}
    &\normLigne{r(t,x) - \{-f(t,x) + g(t, \bfX_t)^2\nabla \log p_t(x) \}}^2\\
    & \qquad = \normLigne{r(t,x) + f(t, x)}^2 -2 g(t, \bfX_t)^2\langle r(t,x), \nabla \log p_t(x) \rangle_\M + g(t, \bfX_t)^4\normLigne{\nabla \log p_t(x)}^2 - 2 g(t, \bfX_t)^2\langle f(t,x), \nabla \log p_t(x) \rangle_\M . 
  \end{align}
  Hence, we get that
  $b(t, \cdot) = \argmin \ensembleLigne{\expeLigne{\norm{f(t, \bfX_t) +
        r(\bfX_t)}^2 - 2 g(t, \bfX_t)^2\langle r(\bfX_t), \nabla \log p_t(\bfX_t) \rangle_\M}}{r
    \in \XM}$.
Using the
      divergence theorem \cite[see][p.51]{lee2018introduction}, we have for any $r \in \XM$
      \begin{align}
        \expeLigne{\langle r(\bfX_t), \nabla \log p_t(\bfX_t) \rangle_\M} &= \textstyle{\int_\M \langle r(x_t), \nabla \log p_t(x_t) \rangle_\M p_t(x_t) \rmd \piinv(x_t)} \\
                                                                       &= - \textstyle{\int_\M \dive(r)(x_t)  p_t(x_t) \rmd \piinv(x_t) = -\expeLigne{\dive(r)(\bfX_t)}}  ,
      \end{align}
which concludes the proof.  
\end{proof}

\begin{figure*}[t!]
    \centering
    \begin{subfigure}[b]{0.24\textwidth}
        \centering
        \includegraphics[height=1.2in]{./images/SB_interpolation/vmf_0.png}
    \end{subfigure}%
    \begin{subfigure}[b]{0.24\textwidth}
        \centering
        \includegraphics[height=1.2in]{./images/SB_interpolation/vmf_30.png}
    \end{subfigure}%
    \begin{subfigure}[b]{0.24\textwidth}
        \centering
        \includegraphics[height=1.2in]{./images/SB_interpolation/vmf_60.png}
    \end{subfigure}%
    \begin{subfigure}[b]{0.24\textwidth}
        \centering
        \includegraphics[height=1.2in]{./images/SB_interpolation/vmf_99.png}
    \end{subfigure}%
    \caption{VMF Interpolation: backward at IPF convergence: left to right}
\end{figure*}

\begin{figure*}[t!]
    \centering
    \begin{subfigure}[b]{0.3\textwidth}
        \centering
        \includegraphics[height=1.2in]{./images/SB_convergence/0.png}
        \caption{Data Sample}
    \end{subfigure}%
    \begin{subfigure}[b]{0.3\textwidth}
        \centering
        \includegraphics[height=1.2in]{./images/SB_convergence/backward_0_final.png}
        \caption{IPF 1}
    \end{subfigure}
    \begin{subfigure}[b]{0.3\textwidth}
        \centering
        \includegraphics[height=1.2in]{./images/SB_convergence/backward_1_final.png}
        \caption{IPF 2}
    \end{subfigure}
    \caption{Interpolation between two VMF: convergence of final sample after multiple IPF steps}
\end{figure*}

\begin{figure*}[t!]
    \centering
    \begin{subfigure}[b]{0.24\textwidth}
        \centering
        \includegraphics[height=1.2in]{./images/SB_interpolation/sh_b0.png}
    \end{subfigure}%
    \begin{subfigure}[b]{0.24\textwidth}
        \centering
        \includegraphics[height=1.2in]{./images/SB_interpolation/sh_b30.png}
    \end{subfigure}%
    \begin{subfigure}[b]{0.24\textwidth}
        \centering
        \includegraphics[height=1.2in]{./images/SB_interpolation/sh_b60.png}
    \end{subfigure}%
    \begin{subfigure}[b]{0.24\textwidth}
        \centering
        \includegraphics[height=1.2in]{./images/SB_interpolation/sh_b99.png}
    \end{subfigure}%
    \caption{Spherical Harmonics: Backward, left to right}
\end{figure*}

\begin{figure*}[t!]
    \centering
    \begin{subfigure}[b]{0.24\textwidth}
        \centering
        \includegraphics[height=1.2in]{./images/SB_interpolation/sh_f0.png}
    \end{subfigure}%
    \begin{subfigure}[b]{0.24\textwidth}
        \centering
        \includegraphics[height=1.2in]{./images/SB_interpolation/sh_f30.png}
    \end{subfigure}%
    \begin{subfigure}[b]{0.24\textwidth}
        \centering
        \includegraphics[height=1.2in]{./images/SB_interpolation/sh_f60.png}
    \end{subfigure}%
    \begin{subfigure}[b]{0.24\textwidth}
        \centering
        \includegraphics[height=1.2in]{./images/SB_interpolation/sh_f99.png}
    \end{subfigure}%
    \caption{Spherical Harmonics: Forward, left to right}
\end{figure*}
% Once we have defined general score-based generative moedls on compact Riemannian
% manifolds, these models can be used as the basis for several extensions. We list
% two of them: conditional sampling and Schr\"odinger bridge. 

% \paragraph{Conditional sampling} We first consider inverse problems on the
% manifold $\M$. Namely, given an observation $y$, we aim at recovering the
% initial signal $x \in \M$. Inverse problems on manifolds are ubiquitous in

%%% Local Variables:
%%% mode: latex
%%% TeX-master: "../main"
%%% End:
